# Supplementary material for: Developing Training Procedures for Piecewise-linear Spline Activation Functions in Neural Networks
Source: arXiv:2509.18161 source file (2025-09-17)
Supplement: Supplementary file 1 [file appendix.tex]

\subsection{Models}

\subsubsection{Regression Models}
\label{apx:regression_models}

The models implemented are simple, feedforward neural nets. For the B-spline version, we simply replace the ReLU activations with B-splines on line 8. 

\lstset{style=mystyle}
\lstinputlisting[language=Python]{code/regression_models.py}

\subsubsection{Regression Model Profiles}
\label{apx:cal_l123}

\begin{table}[ht]
    \centering
    \caption{Performance metrics for 1-layer models.}
    \label{tab:models}
    \begin{tabular}{lrrr}
        \toprule
        Model Architecture & Param count & FLOPs/input & $\mu$s/input \\
        \midrule
        ReLU [48]   & 481 & 912  & 5.66  \\
        B-spline [36] & 469 & 1404 & 16.98 \\
        ReLU [24]    & 241 & 456  & 5.18  \\
        B-spline [19] & 248 & 741  & 14.38 \\
        ReLU [12]   & 121 & 228  & 3.76  \\
        B-spline [9] & 118 & 351  & 12.73 \\
        ReLU [8]    & 81  & 152  & 3.84  \\
        B-spline [6] & 79  & 234  & 12.93 \\
        \bottomrule
    \end{tabular}
\end{table}

\begin{table}[ht]
    \centering
    \caption{Performance metrics for 2-layer models.}
    \label{tab:models_2}
    \begin{tabular}{lrrr}
        \toprule
        Model Architecture & Param count & FLOPs/input & $\mu$s/input \\
        \midrule
        ReLU [48, 24]    & 1.63k & 3192 & 10.34 \\
        B-spline [44, 22] & 1.61k & 4070 & 35.05 \\
        ReLU [24, 12]    & 529    & 1020 & 10.26 \\
        B-spline [22, 10] & 535    & 1484 & 31.95 \\
        ReLU [12, 6]    & 193    & 366  & 6.24  \\
        B-spline [10, 5] & 196    & 585  & 24.09 \\
        ReLU [8, 4]   & 113    & 212  & 6.08  \\
        B-spline [6, 3]   & 106    & 327  & 24.88 \\
        \bottomrule
    \end{tabular}
\end{table}

\begin{table}[ht]
    \centering
    \caption{Performance metrics for 3-layer models.}
    \label{tab:models_3}
    \begin{tabular}{lrrr}
        \toprule
        Model Architecture & Param count & FLOPs/input & $\mu$s/input \\
        \midrule
        ReLU [48, 24, 12] & 1.92k & 3756 & 12.34 \\
        B-spline [44, 22, 11] & 1.88k & 4763 & 43.69 \\
        ReLU [24, 12, 6]  & 601 & 1158 & 11.15 \\
        B-spline [21, 11, 5]  & 608 & 1695 & 39.83 \\
        ReLU [12, 6, 3]  & 211 & 399  & 8.30  \\
        B-spline [10, 5, 2] & 211  & 641  & 34.95 \\
        ReLU [8, 4, 2] & 121    & 226  & 8.47  \\
        B-spline [6, 3, 2] & 119  & 379  & 35.00 \\
        \bottomrule
    \end{tabular}
\end{table}
